# Supplementary material for: Parameter space investigation for spin-dependent electron diffraction in the Kapitza-Dirac effect
Source: arXiv:2308.13200 ancillary file (2023-11-25)
Supplement: Supplementary file 1 [file derivative_calculation.pdf]

# Parameter space investigation for spin-dependent electron diffraction in the Kapitza-Dirac effect Supplemental Material

Yang Wang and Sven Ahrens

August 25, 2023

# Derivative calculation for the algorithm

## 1 Declaration of procedure details

The two orthogonal spinors on the Bloch sphere

$$\psi^A = \begin{pmatrix} \cos\frac{\alpha}{2} \\ \sin\frac{\alpha}{2} e^{i\varphi} \end{pmatrix} \tag{1a}$$

$$\psi^B = \begin{pmatrix} \sin\frac{\alpha}{2} e^{-i\varphi} \\ -\cos\frac{\alpha}{2} \end{pmatrix} \tag{1b}$$

are to be applied at the matrix

$$M = \begin{pmatrix} a_{1,1} + ib_{1,1} & a_{1,2} + ib_{1,2} \\ a_{2,1} + ib_{2,1} & a_{2,2} + ib_{2,2} \end{pmatrix} . \tag{2}$$

From there, we compute the fraction

$$C = \mathcal{C}'(M) = \frac{|M\psi^A|^2}{|M\psi^B|^2} = \frac{A}{B} , \tag{3}$$

with the abbreviations

$$A = |M\psi^A|^2 \tag{4a}$$

$$B = |M\psi^B|^2 \tag{4b}$$

and $C = \mathcal{C}'(M)$. According to the conventions in the main text, we call $\mathcal{C}'(M)$ to be the contrast $\mathcal{C}(M)$, if the variables $\alpha$ and $\varphi$ in Eq. (1) are chosen such that $\mathcal{C}'(M)$ is at the global minimum. The minimum of $C$ is found by in an iterative Newton procedure, for which some of the first, second and mixed derivatives

of $C$ with respect to $\alpha$ and $\varphi$ need to be known. The computation of these derivatives can be abbreviated in terms of the constants

$$C_1 = a_{1,1}^2 + b_{1,1}^2 + a_{2,1}^2 + b_{2,1}^2 \tag{5a}$$

$$C_2 = a_{1,2}^2 + b_{1,2}^2 + a_{2,2}^2 + b_{2,2}^2 \tag{5b}$$

$$C_3 = a_{1,1}a_{1,2} + b_{1,1}b_{1,2} + a_{2,1}a_{2,2} + b_{2,1}b_{2,2} \tag{5c}$$

$$C_4 = a_{1,1}b_{1,2} - a_{1,2}b_{1,1} + a_{2,1}b_{2,2} - a_{2,2}b_{2,1}\,. \tag{5d}$$

# 2 Computation of derivatives

We first compute

$$M\psi^B = \begin{pmatrix} a_{1,1} + ib_{1,1} & a_{1,2} + ib_{1,2} \\ a_{2,1} + ib_{2,1} & a_{2,2} + ib_{2,2} \end{pmatrix} \begin{pmatrix} \sin\frac{\alpha}{2} e^{-i\varphi} \\ -\cos\frac{\alpha}{2} \end{pmatrix} \tag{6a}$$

$$= \begin{pmatrix} (a_{1,1} + ib_{1,1}) \sin\frac{\alpha}{2} e^{-i\varphi} - (a_{1,2} + ib_{1,2}) \cos\frac{\alpha}{2} \\ (a_{2,1} + ib_{2,1}) \sin\frac{\alpha}{2} e^{-i\varphi} - (a_{2,2} + ib_{2,2}) \cos\frac{\alpha}{2} \end{pmatrix}\,. \tag{6b}$$

The absolute value squared of $M\psi^B$ can be written as

$$|M\psi^B|^2 = [(a_{1,1} + ib_{1,1}) \sin\frac{\alpha}{2} e^{-i\varphi} - (a_{1,2} + ib_{1,2}) \cos\frac{\alpha}{2}] \tag{7a}$$

$$\times [(a_{1,1} - ib_{1,1}) \sin\frac{\alpha}{2} e^{i\varphi} - (a_{1,2} - ib_{1,2}) \cos\frac{\alpha}{2}] \tag{7b}$$

$$+ [(a_{2,1} + ib_{2,1}) \sin\frac{\alpha}{2} e^{-i\varphi} - (a_{2,2} + ib_{2,2}) \cos\frac{\alpha}{2}] \tag{7c}$$

$$\times [(a_{2,1} - ib_{2,1}) \sin\frac{\alpha}{2} e^{i\varphi} - (a_{2,2} - ib_{2,2}) \cos\frac{\alpha}{2}] \tag{7d}$$

$$= (a_{1,1}^2 + b_{1,1}^2) \sin^2\frac{\alpha}{2} + (a_{1,2}^2 + b_{1,2}^2) \cos^2\frac{\alpha}{2} \tag{7e}$$

$$- [\cos\varphi (a_{1,1}a_{1,2} + b_{1,1}b_{1,2}) - \sin\varphi (a_{1,1}b_{1,2} - a_{1,2}b_{1,1})] \sin\alpha \tag{7f}$$

$$+ (a_{2,1}^2 + b_{2,1}^2) \sin^2\frac{\alpha}{2} + (a_{2,2}^2 + b_{2,2}^2) \cos^2\frac{\alpha}{2} \tag{7g}$$

$$- [\cos\varphi (a_{2,1}a_{2,2} + b_{2,1}b_{2,2}) - \sin(\varphi) (a_{2,1}b_{2,2} - a_{2,2}b_{2,1})] \sin\alpha \tag{7h}$$

$$= C_1 \sin^2\frac{\alpha}{2} + C_2 \cos^2\frac{\alpha}{2} - (C_3 \cos\varphi - C_4 \sin\varphi) \sin\alpha\,. \tag{7i}$$

Similarly, for $M\psi^A$ we obtain

$$|M\psi^A|^2 = C_1 \cos^2\frac{\alpha}{2} + C_2 \sin^2\frac{\alpha}{2} + (C_3 \cos\varphi + C_4 \sin\varphi) \sin\alpha\,. \tag{8}$$

Now we compute the derivatives of $C$, which we express in terms of $A = |M\psi^A|^2$ and $B = |M\psi^B|^2$:

- First derivative of $C$ with respect to $\alpha$

$$\frac{\partial}{\partial\alpha} C = \frac{\partial}{\partial\alpha} (A \cdot B^{-1}) = \frac{\partial}{\partial\alpha} A \cdot B^{-1} - AB^{-2} \frac{\partial}{\partial\alpha} B \tag{9}$$

- Second derivative of $C$ with respect to $\alpha$

$$\frac{\partial^2}{\partial^2\alpha}C = \frac{\partial^2}{\partial^2\alpha}A \cdot B^{-1} - 2\frac{\partial}{\partial\alpha}AB^{-2}\frac{\partial}{\partial\alpha}B + 2AB^{-3}\frac{\partial^2}{\partial\alpha^2}B - AB^{-2}\frac{\partial^2}{\partial\alpha^2}B \tag{10}$$

- First derivative of $C$ with respect to $\varphi$

$$\frac{\partial}{\partial\varphi}C = \frac{\partial}{\partial\varphi}(AB^{-1}) = \frac{\partial}{\partial\varphi}AB^{-1} - AB^{-2}\frac{\partial}{\partial\varphi}B \tag{11}$$

- Second derivative of $C$ with respect to $\varphi$

$$\frac{\partial^2}{\partial^2\varphi}C = \frac{\partial^2}{\partial^2\varphi}AB^{-1} - 2\frac{\partial}{\partial\varphi}AB^{-2}\frac{\partial}{\partial\varphi}B \tag{12a}$$

$$+ 2AB^{-3}\frac{\partial^2}{\partial\varphi^2}B - AB^{-2}\frac{\partial^2}{\partial\alpha\partial\varphi}B \tag{12b}$$

- Mixed derivative of $C$ with respect to $\alpha$ and $\varphi$

$$\frac{\partial^2}{\partial\alpha\partial\varphi}C = \frac{\partial^2}{\partial\alpha\partial\varphi}AB^{-1} - \frac{\partial}{\partial\alpha}AB^{-2}\frac{\partial}{\partial\varphi}B - \frac{\partial}{\partial\varphi}AB^{-2}\frac{\partial}{\partial\alpha}B \tag{13a}$$

$$+ 2AB^{-3}\frac{\partial}{\partial\alpha}B\frac{\partial}{\partial\varphi}B - AB^{-2}\frac{\partial^2}{\partial\alpha\partial\varphi}B \tag{13b}$$

$$= \frac{\partial^2}{\partial\alpha\partial\varphi}AB^{-1} - 2B^{-2}\left(\frac{\partial}{\partial\alpha}A\frac{\partial}{\partial\varphi}B + \frac{\partial}{\partial\alpha}B\frac{\partial}{\partial\varphi}A\right) \tag{13c}$$

$$+ 2AB^{-3}\frac{\partial}{\partial\alpha}B\frac{\partial}{\partial\varphi}B - AB^{-2}\frac{\partial^2}{\partial\alpha\partial\varphi}B \tag{13d}$$

The derivatives of $C$ are now expressed in terms of derivatives of $A$ and $B$. Consequently, we are computing the derivatives of $A$ now.

- First derivative of $A$ with respect to $\alpha$

$$\frac{\partial}{\partial\alpha}A = -C_1\cos\frac{\alpha}{2}\sin\frac{\alpha}{2} + C_2\sin\frac{\alpha}{2}\cos\frac{\alpha}{2} + C_3\cos\alpha\cos\varphi + C_4\cos\alpha\sin\varphi$$

$$= -\frac{1}{2}(C_1 - C_2)\sin\alpha + C_3\cos\alpha\cos\varphi + C_4\cos\alpha\sin\varphi \tag{14}$$

- Second derivative of $A$ with respect to $\alpha$

$$\frac{\partial^2}{\partial\alpha^2}A = -\frac{1}{2}(C_1 - C_2)\cos\alpha - C_3\sin\alpha\cos\varphi - C_4\sin\alpha\cos\varphi \tag{15}$$

- First derivative of $A$ with respect to $\varphi$

$$\frac{\partial}{\partial\varphi}A = -C_3\sin\alpha\sin\varphi + C_4\sin\alpha\cos\varphi \tag{16}$$

- Second derivative of $A$ with respect to $\varphi$

$$\frac{\partial^2}{\partial\varphi^2}A = -C_3 \sin\alpha\cos\varphi - C_4 \sin\alpha\sin\varphi \tag{17}$$

- Mixed derivative of $A$ with respect to $\varphi$

$$\frac{\partial^2}{\partial\alpha\partial\varphi}A = -C_3 \cos\alpha\sin\varphi + C_4 \cos\alpha\cos\varphi \tag{18}$$

The derivatives of $B$ are computed similarly:

- First derivative of $B$ with respect to $\alpha$

$$\frac{\partial}{\partial\alpha}B = \frac{1}{2}(C_1 - C_2)\sin\alpha - (\cos\varphi C_3 - \sin\varphi C_4)\cos\alpha \tag{19}$$

- Second derivative of $B$ with respect to $\alpha$

$$\frac{\partial^2}{\partial\alpha^2}B = \frac{1}{2}(C_1 - C_2)\cos\alpha + (\cos\varphi C_3 - \sin\varphi C_4)\sin\alpha \tag{20}$$

- First derivative of $B$ with respect to $\varphi$

$$\frac{\partial}{\partial\varphi}B = \sin\varphi\cos\alpha C_3 + cos\varphi\sin\alpha C_4 \tag{21}$$

- Second derivative of $B$ with respect to $\varphi$

$$\frac{\partial^2}{\partial\varphi^2}B = \cos\varphi\sin\alpha C_3 - \sin\varphi\sin\alpha C_4 \tag{22}$$

- Mixed derivative of $B$ with respect to $\varphi$

$$\frac{\partial^2}{\partial\alpha\partial\varphi}B = \sin\varphi\cos\alpha C_3 + \cos\varphi\cos\alpha C_4 \tag{23}$$
